# Supplementary material for: LLM as Dataset Analyst: Subpopulation Structure Discovery with Large Language Model
Source: arXiv:2405.02363 source file (2024-07-24)
Supplement: Supplementary file 1 [file X_suppl.tex]

%%%%%%%%%%%%%%%%%%%%%%% Overview %%%%%%%%%%%%%%%%%%%
\section{Supplementary Overview}
To provide comprehensive details of our methods and experiments, we further elaborate the theoretical analysis of the Criteria Refinement and present more details and results of experiments in the supplementary material. The additional content is presented from the following perspectives.

\begin{itemize}
    \item Terminologies

    - Definitions of the terminologies used in this paper
    \item Theoretical Analysis

    - Theoretical demonstration of the effectiveness for the self-consistency indicator in Criteria Refinement
    \item Supplementary Related Work
    
    - Expanded related work about subpopulation shift

    - Expanded related work about dataset bias discovery
    \item Supplementary Experiment Analysis

    - Experiment setup details for subpopulation structure discovery, long tail attribute identification, slice discovery and slice prediction

    - Visualization results of subpopulation structure discovery, long tail attribute identification, and slice discovery
    
\end{itemize}

%%%%%%%%%%%%%%%%%%%%%%% Terminologies %%%%%%%%%%%%%%%%%%%
\section{Terminologies}
The terminologies used in this paper are given in the table \ref{tab:terminologies}, providing clear definitions of all the concepts introduced in this paper. 
\begin{table}[H]
    \centering
    \begin{tabularx}{\textwidth}{l|X}
        \toprule
        \makecell{Terminologies} & \makecell{Definitions}   \\
        \hline
        \makecell{Language Space} &  The language space $\mathbb{Z}$ is the set of valid sentences in a language.\\
        \hline
        \makecell{Attribute} & An attribute $a$ of an image is a description of the image in $\mathbb{Z}$ 
        about one aspect of this image.\\
        \hline
        \makecell{Dimension} &  A dimension is a function $f$ defined on the dataset $\mathbb{D}$ that projects one image $s$ to its corresponding attribute $a$. $f: \mathbb{D}\mapsto\mathbb{Z}$.A dimension $f$ can have several attributes $A_f=\{f(s)| s\in\mathbb{D}\}$.\\
        \hline
        \makecell{Criteria} &  A criteria is a tuple of $(\mathbb{F},\mathbb{A})$, where $\mathbb{F}=\{f_i| i=1,2,...M\}$ is the set of dimensions, and $\mathbb{A}=\{A_f| f\in \mathbb{F}\}$ contains the sets of attributes corresponding to the dimensions.\\
        \hline
        \makecell{Subpopulation} & A subpopulation $s$ of an image dataset $\mathbb{D}$ is a subset of the dataset that share several common characteristics, $f_i, i=1,2,3...k$. $s=\{d|d\in \mathbb{D}; s.t.\forall i=1,2,3...k, f_i(d)\equiv a_i\}$\\
        \hline
        \makecell{Subpopulation Structure} & A subpopulation structure of an image dataset is a tuple of $(\mathbb{S},\mathbb{X})$,where $\mathbb{S}$ is the set of subpopulations of $\mathbb{D}$, and $\mathbb{X}$ is their hierarchical relations of inclusion, $\mathbb{X} = \{(s_1,s_2)|s_1,s_2\in \mathbb{S};  s_1 \subset s_2\}$.\\
        \hline
        \makecell{Subpopulation Shift} & Subpopulation shift refers to the distributional shift between the training data $\mathbb{D}_{train}$ and the testing data $\mathbb{D}_{test}$ in special cases when the shift is several alternations of subpopulations $\mathbb{D}_{train}\Delta\mathbb{D}_{test}=\cup_i s_i; s.t. s_t \in \mathbb{S}$.\\
        \bottomrule
    \end{tabularx}
    % \vspace{2mm}
    \caption{The definitions of the terminologies defined in the paper.}
    \label{tab:terminologies}
\end{table}

%%%%%%%%%%%%%%%%%%%%%%% Theoretical Analysis %%%%%%%%%%%%%%%%%%%
\section{Theoretical Analysis}
The proposed method undergoes a lengthy refining process to ensure that the generated criteria effectively cover a wide range of images. To assess whether a criterion is well-suited for the dataset, we introduce the concept of \textbf{classification success probability}. Intuitively, a well-suited criterion has a high probability of correctly classifying an image sample from the dataset without triggering further refinement. We denote this indicator as $W(m,c)$, where $W(m,c)=0$ if the criterion $c$ fails to classify image $m$ accurately and $W(m,c)=1$ if it succeeds without triggering refinement. The overall effectiveness of a criterion can be evaluated by its \textbf{expected classification success probability}, denoted as $W(c)=\mathbb{E}m W(m,c)$, which represents the expected classification success rate across all images. Utilizing Monte Carlo estimation, we approximate $W(c)$ with $W_n(c)=\frac{1}{n}\sum_i W(m_i,c)$, where $m_i$ represents the $i$th image sample. By applying the law of large numbers and the central limit theorem, we can establish that $\lim{n\to\infty} W_n(c)=W(c)$. Our stopping criterion, which halts refinement after $N$ consecutive iterations without refinement, serves as theoretical support for ensuring that $W(c)$ remains relatively large throughout refining process.

%%%%%%%%%%%%%%%%%%%%%%% Supplementary Related Work %%%%%%%%%%%%%%%%%%%
\section{Supplementary Related Work}
\label{Supplementary Related Work}

\subsection{Dataset Bias Discovery}
Datasets can contain various types of bias~\cite{fabbrizzi2022survey}, such as selection bias~\cite{torralba2011unbiased}, framing bias~\cite{torralba2011unbiased}, spurious correlation~\cite{lynch2023spawrious}, contextual bias~\cite{singh2020context_bias, liang2022metashift} and so on. These biases can diminish the model's generalization and reliability, leading to the biases and fairness issues~\cite{fabbrizzi2022survey}. Several methods have been developed to identify these biases in visual datasets~\cite{fabbrizzi2022survey, dulhanty2019auditing, shankar2017no, jang2019quantification, wang2022revise}. One of the methods that is most relevant to ours is reduction to tabular data~\cite{fabbrizzi2022survey}, which measures biases after transforming images into a tabular format. Dulhanty et al. ~\cite{dulhanty2019auditing} assesses gender and age bias in ImageNet subsets~\cite{russakovsky2015imagenet} after applying corresponding recognition models. Shankar et al. ~\cite{shankar2017no} detects geographic bias from the textual information and URL metadata of ImageNet\cite{russakovsky2015imagenet} and Open Images\cite{kuznetsova2020open}. Jang et al.~\cite{jang2019quantification} identifies gender bias in movies by computing eight quantitative metrics, such as emotional diversity and spatial occupancy, using face attributes extracted via the Microsoft Face API. REVISE~\cite{wang2022revise} is a  comprehensive tool for discovering dataset biases, focusing on object-based, person-based, and geography-based analysis. Object-based analysis examines object count, scale, co-occurrence, scene diversity, and appearance diversity. The analysis about count, scale and co-occurrence of objects relies on the manual annotation like bounding box~\cite{lin2014coco}. Scene attributes are inferred using a scene recognition model trained on Places~\cite{zhou2017places}, and the appearance of each instance is represented by features from a pretrained classification model. 

Although current methods have made some progress in discovering dataset bias, they face several limitations. Some depend on manual annotations~\cite{wang2022revise} or metadata~\cite{shankar2017no}, restricting their use in image classification datasets that have only class-level annotations. Moreover, most methods can only deal with a single~\cite{shankar2017no} or a limited number~\cite{dulhanty2019auditing, jang2019quantification, wang2022revise} of bias dimensions, lack of generality to comprehensively analyze various biases~\cite{zhang2022nico, liang2022metashift, lynch2023spawrious}. For general objects, tools like REVISE~\cite{wang2022revise} only considers generic bias dimensions like scenes and co-occurrence objects, but neglects specific dimensions relevant to different classes~\cite{zhang2022nico}. For example, the 'posture' dimension needs to be considered for the class 'dog' but not for 'flower' or 'car'. Additionally, REVISE lacks the capability to evaluate fine-grained, class-specific attribute biases like appearance bias in a interpretable way, due to the absence of a model that can recognize such attributes. 

Overall, existing methods can't discover different types of bias in visual datasets automatically in a unified manner. In this work, we propose a general paradigm to discover the subpopulation structure within visual datasets. This framework can be employed to evaluate biases by quantifying the proportions of different subpopulations. The "MLLM caption + LLM summary" approach automatically extracts and organizes various attributes from images without requiring human intervention or diverse visual expert models, effectively solving the previously mentioned issues.

% \subsection{ICTC}

\subsection{Subpopulation Shift}
Machine learning models often encounter performance degradation due to subpopulation shift~\cite{izmailov2022feature,joshi2022spurious, Geirhos_2020shortcut}. This issue arises when the distribution of subpopulations varies significantly between training and testing datasets~\cite{cai2021theory,koh2021wilds}. Subpopulation shift encompasses four primary categories~\cite{yang2023change}: spurious correlations~\cite{Geirhos_2020shortcut}, attribute imbalance~\cite{martinez2021blind}, class imbalance~\cite{liu2019class_imbalance}, and attribute generalization~\cite{santurkar2020attribute_generalization}. Spurious correlations occur when an attribute incorrectly correlates with the label in training but not in test data~\cite{yang2023change, Geirhos_2020shortcut}. Attribute imbalance arises when certain attributes are much less common than others~\cite{yang2023change, martinez2021blind, tang2022intra_class_long_tail}. Class imbalance is noticeable when class labels are unevenly distributed, often resulting in bias against less represented classes~\cite{yang2023change, liu2019class_imbalance}. Lastly, in some cases, certain attributes might be absent in the training data but present in the test data for specific categories, leading to the challenge of attribute generalization~\cite{santurkar2020attribute_generalization}. 

There are many relevant methods to solve the problem. 
% Subgroup Robust Methods
For \textit{Subgroup Robust Methods}, GroupDRO~\cite{sagawa2019distributionally} employs strong regularization to improve the worst-group performance of Distributionally Robust Optimization (DRO) when applied to overparameterized neural networks. LfF~\cite{nam2020learning} identifies distinct loss value patterns between samples with spurious correlations and those without during training. It subsequently trains a secondary model with weighted cross entropy loss leveraging this insight, facilitating balanced feature learning from both types of samples. JTT~\cite{liu2021just} initially identifies the misclassified samples in the training set by the ERM model and subsequently increases the weights of these samples to train a debiasing model. LISA~\cite{yao2022improving} introduces intra-label and intra-domain mixup techniques to mitigate spurious correlations in data, facilitating the learning of domain-invariant predictors without explicit regularization constraints.
% Imbalanced Learning
For \textit{Imbalanced Learning},  ReSample~\cite{japkowicz2000class} modifies the sampling rates across classes with varying frequencies to balance the contribution of  each class during training. ReWeight~\cite{japkowicz2000class} adjusts the loss function weights based on class frequencies. In subpopulation shift, rare subgroups often correspond to hard examples in training. Focal Loss~\cite{lin2017focal} offers a solution to this issue by introducing a modulating factor into the cross-entropy loss, amplifying the contribution of hard samples. CBLoss~\cite{cui2019class} adjusts the loss weighting based on the effective number of samples per class. Bsoftmax~\cite{ren2020balanced} derives the balanced softmax for addressing long-tail distribution issues and proposes meta sampler to mitigate the over-balancing problem.
% Data Augmentation
For \textit{Data Augmentation}, standard Mixup~\cite{zhang2017mixup} demonstrates grea performance across various datasets~\cite{yang2023change}.

Despite the variety of available methods, recent findings~\cite{yang2023change} indicate that while current approaches can alleviate spurious correlations and class imbalances, they inadequately address attribute imbalance and attribute generalization, suggesting an absence of unified methods for all subpopulation shifts. Designing universally applicable methods in a model-centric way remains challenging due to the variability of mathematical models for diverse settings.

To address these challenges, we rethink the task from a data-centric perspective. We  observe that all four types of subpopulation shift closely correlate with the subpopulation distribution of dataset, and the primary challenge lies in the limited understanding of these distribution within the dataset~\cite{yang2023change}. To tackle this problem, we leverage the capabilities of LLM and MLLM, and construct an automated pipeline, SSD-LLM, to comprehensively analyze the subpopulation structure of the dataset, characterizing the distribution in a interpretable manner. The proposed method enhances our understanding of the attribute distribution in the dataset, paving the way for solving subpopulation shifts problem using data-centric methods, such as synthetic data generation~\cite{dunlap2023diversify}.

\subsection{Slice Discovery}

Machine learning models often make systematic errors in specific data subgroups (or \textit{slices})~\cite{eyuboglu2022domino}. To identify model's underperforming slices, numerous slice discovery methods(SDMs) have been proposed~\cite{d2022spotlight, eyuboglu2022domino, gao2023adaptive, yenamandra2023facts}. These methods generally consist of three steps~\cite{eyuboglu2022domino}: (1) embedding input data in a representation space, (2) identifying underperforming slices using clustering or dimensionality reduction techniques, and (3) describe the clusters using natural language. In the last step, cluster explanations can be categorized into three approaches: human examination~\cite{d2022spotlight, gao2023adaptive}, matching phrase from a pre-generated corpus through image and text embedding similarity~\cite{eyuboglu2022domino}, and keyword extraction from image captions~\cite{yenamandra2023facts}. However, these methods have several limitations, such as dependent on human participation~\cite{d2022spotlight, gao2023adaptive}, inconsistent slice identification~\cite{eyuboglu2022domino}, and focusing on the absolute count of visual attributes~\cite{d2022spotlight, eyuboglu2022domino, yenamandra2023facts}. In this work, we design task-specific prompts for the slice discovery task after identifying the subpopulation structure of test sets. Specifically, we compute the error rate for each attribute and select TopK attributes with the highest error rates. Then LLM is used to generate concise and coherent slice topics from these attributes and the category name. Compared to previous work, we have three advantages: (1) full-automatically, (2) considers various dimensions and attributes, and (3) analyzes slices based on the error rates rather than the counts of attributes. This results in more coherent and accurate identification of model weaknesses.

%%%%%%%%%%%%%%%%%%%%%%% Supplementary Experiment Analysis %%%%%%%%%%%%%%%%%%%

\section{Supplementary Experiment Analysis}
\subsection{Experiment Details}

\subsubsection{Dataset Subpopulation Organization}

Organizing the subpopulation within datasets refers to the task of exploring the dataset and identifying the latent subpopulation structures. % What is SSD
inappropriateThis task enables hierarchical organization for the dataset, provides valuable insights that can deepen our understanding of the dataset, and supports predictions about where models trained with this dataset might underperform. % Why matter

Subpopulation structure discovery entails systematical intra-class labeling of the dataset, which more specifically requires discovering latent classification dimensions and corresponding attributes. % Analysis

\noindent {\textbf{Setup}}
The aforementioned attributes serve as secondary labels for the dataset. The original dataset's secondary labels are treated as ground truth (GT) labels. The assessment involves matching assigned secondary labels with GT labels through text similarity, checking for the nearest GT label for each secondary label, and calculating the image pairing accuracy between the assigned secondary labels and the corresponding GT labels. The overall clustering accuracy, representing the subgroup structure quality, is then determined by the ratio of correctly paired images to total number of images in the dataset. 

The study employs the Stanford 40 Action Dataset~\cite{yao2011human}, comprising 9,532 images depicting individuals engaged in diverse actions, annotated across 40 distinct action classes such as singing, dancing, and reading. To enrich the analysis, we introduce two additional label collections following~\cite{kwon2023image}.  

\noindent {\textbf{Comparison Methods}}
Scan~\cite{van2020scan} is executed via a bifurcated methodology, wherein feature extraction and clustering operations are distinctly separated. Initially, the task of representation learning, conducted in a self-supervised manner, is employed to extract semantic features. Subsequently, within learnable clustering frameworks, these extracted features serve as priors for the clustering process. This methodology decouples the direct reliance of clustering on underlying features, a characteristic prevalent in contemporary end-to-end learning models. IC|TC~\cite{kwon2023ictc} introduces a proposed methodology for image clustering, which utilizes contemporary vision-language models alongside large language models. This approach enables clustering based on criteria defined by textual descriptions provided by users. It signifies a shift in the paradigm of image clustering by requiring minimal yet practical human intervention. In exchange, it offers users enhanced control over the outcomes of the clustering process.

\noindent {\textbf{Results}}
% 我们分别对狗、猫、车进行了若干组实验结果的可视化，可以看到每一个 attribute 下与之对应的图像都与其高度一致。值得一提的是，我们想强调指出在狗这一类，activity 这个维度中，我们的方法discovery出了playing and running 两个维度，这在图像中是由狗狗是否有玩具等物品得以区分的，可以证明我们的方法属性挖掘的卓越能力和图像assign的匹配程度很高。
As Fig~\ref{fig:appendix1}~\ref{fig:appendix2}, we have visualized the experimental results for different categories including dogs, cats, and cars. The results demonstrate a high consistency of the images under each attribute. Specifically, for the dog category in the dimension of activity, our method distinguishes between "playing" and "running" based on the presence of toys and other objects in the images. This underscores the outstanding capability of our approach in attribute identification and its high alignment with image categorization.

\subsubsection{Subpopulation Shift}
Subpopulation shift is a common problem when machine learning model meets the occurrences of dismatchings in the training and testing distributions. Our method SSD-LLM can better tackle such situations by discovering the subpopulation structures within datasets and augmenting generated images to the dataset for better performances.

\noindent {\textbf{Datasets}}
We use Metashift~\cite{liang2022metashift} and Waterbirds~\cite{sagawa2019distributionally} as benchmarks. For Metashift, the task is to classify images as "cat" or "dog", the general contexts "indoor / outdoor" have a natural spurious correlation with the class labels. Concretely, in the training data, cat(ourdoor) and dog(indoor) subsets are the minority groups, while cat(indoor) and dog(outdoor) are majority groups. The total size of training data are kept 2276 images unchanged and only the portion of minority groups vary. We use a balanced test set with 874 images to report both average accuracy and worst group accuracy.
For Waterbirds, the task is to classify images of birds as "waterbird" or "landbird", and the label is spuriously correlated with the image background, which is either "land" or "water". We use standard splits train:val:test = 4795: 1199: 5794 given by prior work~\cite{yang2023change}.

\noindent {\textbf{Evaluation Metrics}}
We apply the average \& worst group accuracy (WGA). The average accuracy is defined as the accuracy over all samples. For WGA, we compute the accuracy over all subgroups in the test set and report the worst one. In validation set, we view each class as a subgroup, so WGA degenerates to the worst-class accuracy.

\noindent {\textbf{Model Selection}}
To get close to the reality, we consider the most challenging setting of unknown attributes in both training \& validation in \cite{yang2023change}. When attributes are completely unknown, we use "validation set worst-group accuracy" for model selection, which degenerates to "worst-class accuracy" in this scenario.
 
\noindent {\textbf{Training Details}}
Following ~\cite{yang2023change}, we use pretrained ResNet-50 model~\cite{he2016resnet} as the backbone. We utilize standar image pre-process steps: resize and center crop the image to 224 ×224 pixels, and perform normalization using the ImageNet channel statistics. We use the SGD with momentum as optimizer. We train all models for 5000 steps on Metashift and Waterbirds .

\noindent {\textbf{Comparison Methods}}
Following recent benchmarking efforts~\cite{yang2023change}, we compare SSD-LLM with several types of methods: (1) \textit{vanilla:} ERM~\cite{vapnik1999overview}, (2) \textit{Subgroup Robust Methods:} GroupDRO~\cite{sagawa2019distributionally}, LfF~\cite{nam2020learning}, JTT~\cite{liu2021just}, LISA~\cite{yao2022improving}, (3) \textit{Imbalanced Learning:} ReSample~\cite{japkowicz2000class}, ReWeight~\cite{japkowicz2000class}, Focal~\cite{lin2017focal}, CBLoss~\cite{cui2019class}, Bsoftmax~\cite{ren2020balanced}, (4) \textit{Traditional Data Augmentation:} Mixup~\cite{zhang2017mixup}, RandAug~\cite{cubuk2020randaugment}, (5) \textit{Diffusion:} Class Prompt~\cite{shipard2023diversity}, Class-Attribute Prompt~\cite{shipard2023diversity}, CiP~\cite{lei2023cip}. 
% Appendix contains more details about comparion methods.
Details about the types (2)(3)(4) can be seen in Sec. \ref{Supplementary Related Work}
For diffusion-based methods, we use SDXL-turbo as the text2image model with 4 steps and 0 guidance scale. The text for Class Prompt is \textit{"A photo of a [CLS] in a specific scene"}, for Class-Attribute Prompt is \textit{"A photo of a [CLS] in [ATTR] scene"}, for CiP is \textit{"A photo of [CLS], [Image Caption]"}.

\noindent {\textbf{Hyperparameters Search Protocol}}
To ensure a fair comparison, following~\cite{yang2023change}, we conduct a random search of 16 trials over a joint distribution of all hyperparameters. We then use the validation set to select the best hyperparameters for each algorithm, fix them, and rerun the experiments under five different random seeds to report the final average results. The details of hyperparameter choices for each algorithm are in Table 2.

\begin{table}[H]
\label{appendix:table:hyperparameters}
\small
\begin{center}
% \resizebox{0.9\textwidth}{!}{
\begin{tabularx}{\textwidth}{llll}
\toprule[1.5pt]
\textbf{Condition} & \textbf{Parameter} & \textbf{Default value} & \textbf{Random distribution} \\
\midrule\midrule
\multicolumn{4}{l}{\emph{\textbf{General:}}} \\
\midrule
\multirow{2}{*}{ResNet}     & learning rate & 0.001 & $10^{\text{Uniform}(-4, -2)}$ \\
                            & batch size & 108 & $2^{\text{Uniform}(6, 7)}$ \\

\midrule\midrule
\multicolumn{4}{l}{\emph{\textbf{Algorithm-specific:}}} \\
\midrule
GroupDRO                    & eta & 0.01 & $10^{\text{Uniform}(-3, -1)}$ \\
\midrule

\multirow{2}{*}{JTT}        & first stage step fraction & 0.5 & $\text{Uniform}(0.2, 0.8)$ \\
                            & lambda & 10 & $10^{\text{Uniform}(0, 2.5)}$ \\
\midrule
LfF                         & q & 0.7 & $\text{Uniform}(0.05, 0.95)$ \\
\midrule
\multirow{2}{*}{LISA}       & alpha & 2 & $10^{\text{Uniform}(-1, 1)}$ \\
                            & p\_select & 0.5 & $\text{Uniform}(0, 1)$ \\

\midrule
Focal                       & gamma & 1 & $0.5 * 10^{\text{Uniform}(0, 1)}$ \\
\midrule
CBLoss                      & beta & 0.9999 & $1 - 10^{\text{Uniform}(-5, -2)}$ \\
\midrule
Mixup                       & alpha & 0.2 & $10^{\text{Uniform}(0, 4)}$ \\
\midrule
\bottomrule[1.5pt]
\end{tabularx}
% }
% \vspace{4mm}
\caption{Hyperparameters search space for all experiments.}
\end{center}
% \vspace{-8mm}
\end{table}

% \noindent {\textbf{Our Implementation Details}}

\subsubsection{Slice Discovery}

Slice discovery is a data-driven task aimed at enhancing our understanding of targeted datasets and improving models' performances on it.
This process involves the identification and analysis of unstructured input data to pinpoint semantically meaningful subgroups. These subgroups are characterized by their distinct features, which result in sub-optimal performance by the model. 
 
\noindent {\textbf{Setup}} We initially employ various Slice Discovery Methods(SDMs) to identify error attribute sets within a specific dataset and subsequently form topics in a defined format. These topics are then utilized to perform retrieval on CC3M~\cite{sharma2018conceptual}. We then use Google API to filter the retrieved images, reducing noise that may occur during the process. The filtered images are classified using a designated model, and the resulting error rate from this classification serves as an evaluation metric to reveal the effectiveness of the different SDMs. It's noteworthy that here we adopts a looser failure definition. Because it's still hard for caption models to gain fine-grined information about categroy of single image, we consider one classification case is correct when model can distinguish its super class in Imagenet. 
This comparison is predicated on the premise that if a particular topic or caption, denoted as $t$, accurately encapsulates a flaw within the model, then selecting new samples based on the conditional probability $x \sim  P(X\mid t)$ is expected to result in a substantially higher rate of model failures.

\noindent {\textbf{Implemental Details}}
In our experiment, we conduct a comparison of SDMs in ImageNet classification models, mainly focus on six distinct classes: \{boat, car, cat, dog, bird, truck\} in the validation set of Imagenet~\cite{russakovsky2015imagenet}. Specifically, we define a test as failed if it resulted in a false negative, which occurs when the model fails to correctly identify an object $y$ present in the image $x$, instead incorrectly predicting an object that is not in the image. 
For this evaluation, we utilize the ResNet50~\cite{he2015deep} model to systematically assess these misclassifications across the specified categories.
Based on the test results of pretrain model mentioned above, SSD-LLM utilizes GPT4 to construct a hierarchical structure. The set of attributes having a high error rate, identified through an intersection analysis within the attribute pool(second layer of the tree), is designated as the final topic. 
In our experiment, each method systematically identifies 20 key topics for each category, with a focus on those demonstrated the most frequent failures. To evaluate the failure rate of these specific topics against newly correlated data, we engaged in a retrieval process of the nearest neighbors from the CC3M~\cite{sharma2018conceptual} dataset. For each topic, we retrieved 50 images. This retrieval was conducted using a prompt consist of the topic's name, making the search more effectively.
As for Domino, we equip Bert~\cite{devlin2018bert} to fill template when it caption clusters. All experiments are conducted using the PyTorch~\cite{paszke2019pytorch} library on NVIDIA A100.

\noindent {\textbf{Comparison Methods}}
The general prompt simplifies search queries by directly using  \textit{a photo of \{class\}} as the topic, capitalizing on visual cues for enhanced retrieval precision.
By inputting class labels into GPT, GPT-suggest elicits semantically relevant attributes, optimizing topic-specific retrieval through inferred contextual details.
Domino~\cite{eyuboglu2022domino} is recognized as an advanced method for slice discovery that clusters errors in validation sets and annotates them with auto-generated captions. Specifically, it clusters the validation examples by category using an error-aware Gaussian mixture model in the latent space of the Contrastive Language–Image Pre-training (CLIP) framework. Each cluster is then described with a caption. To enhance the comprehensiveness of our comparisons, we also propose two plain baselines. 
One simulates random outcomes without relying on prior knowledge.This is achieved by querying a LLM about potential attributes (attr) and corresponding values (val) for each class $y$ under consideration.The responses from the LLM are then aggregated into a structured format, denoted as \textit{a photo of \{val\} \{attr\} \{y\}}, which serves as a retrieval topic for next experimental steps. Another is the failure rate on the original ImageNet validation dataset. B2T~\cite{kim2023biastotext}, which interprets visual biases as keywords. The framework detects biases in computer vision models by extracting common keywords from mispredicted image descriptions. It validates these keywords using a visual-language model like CLIP~\cite{radford2021clip}, and applies them to debiasing training, enhancing zero-shot classifiers, comparing model failures, and diagnosing label issues, demonstrating effectiveness across multiple datasets.

In our study, we draw a comparison between the clusters identified by plain baselines, Domino and the topics delineated by SSD-LLM on a non-seen dataset.

\noindent {\textbf{Results}}
% 我们的SSD-LLM可以找出模型表现不好的切片。我们将其根据维度-属性以及topic进行陈列，可以观察到被模型选出来的图像确实具有一定的迷惑性，尤其是Boat类中的slice，即使是人可能也无法很准确的进行判断，可视化结果再一次证明了我们方法的有效性。
As Fig~\ref{fig:appendix3} shows, the average error rate for these selected topics significantly exceed that of the overall categories, illustrating our SSD-LLM can pinpoint specific subsets where the model underperforms. We categorize and present these subsets based on various dimensions, attributes, and topics. It is evident that the images selected by the model are challenging to interpret, especially within the 'Boat' category. Such complexity indicates that these images could challenge even human discernment, highlighting our approach's effectiveness in identifying and examining data subsets that present significant challenges.
\subsection{Supplementary Visualization Experiment}
\newpage
\subsubsection{Dataset Subpopulation Organization}
Here we present more visualization of the subpopulations discovered by the method SSD-LLM in Fig\ref{fig:appendix1} and Fig\ref{fig:appendix2}.
\begin{figure}[H]
    \centering
    \includegraphics[width=1\linewidth]{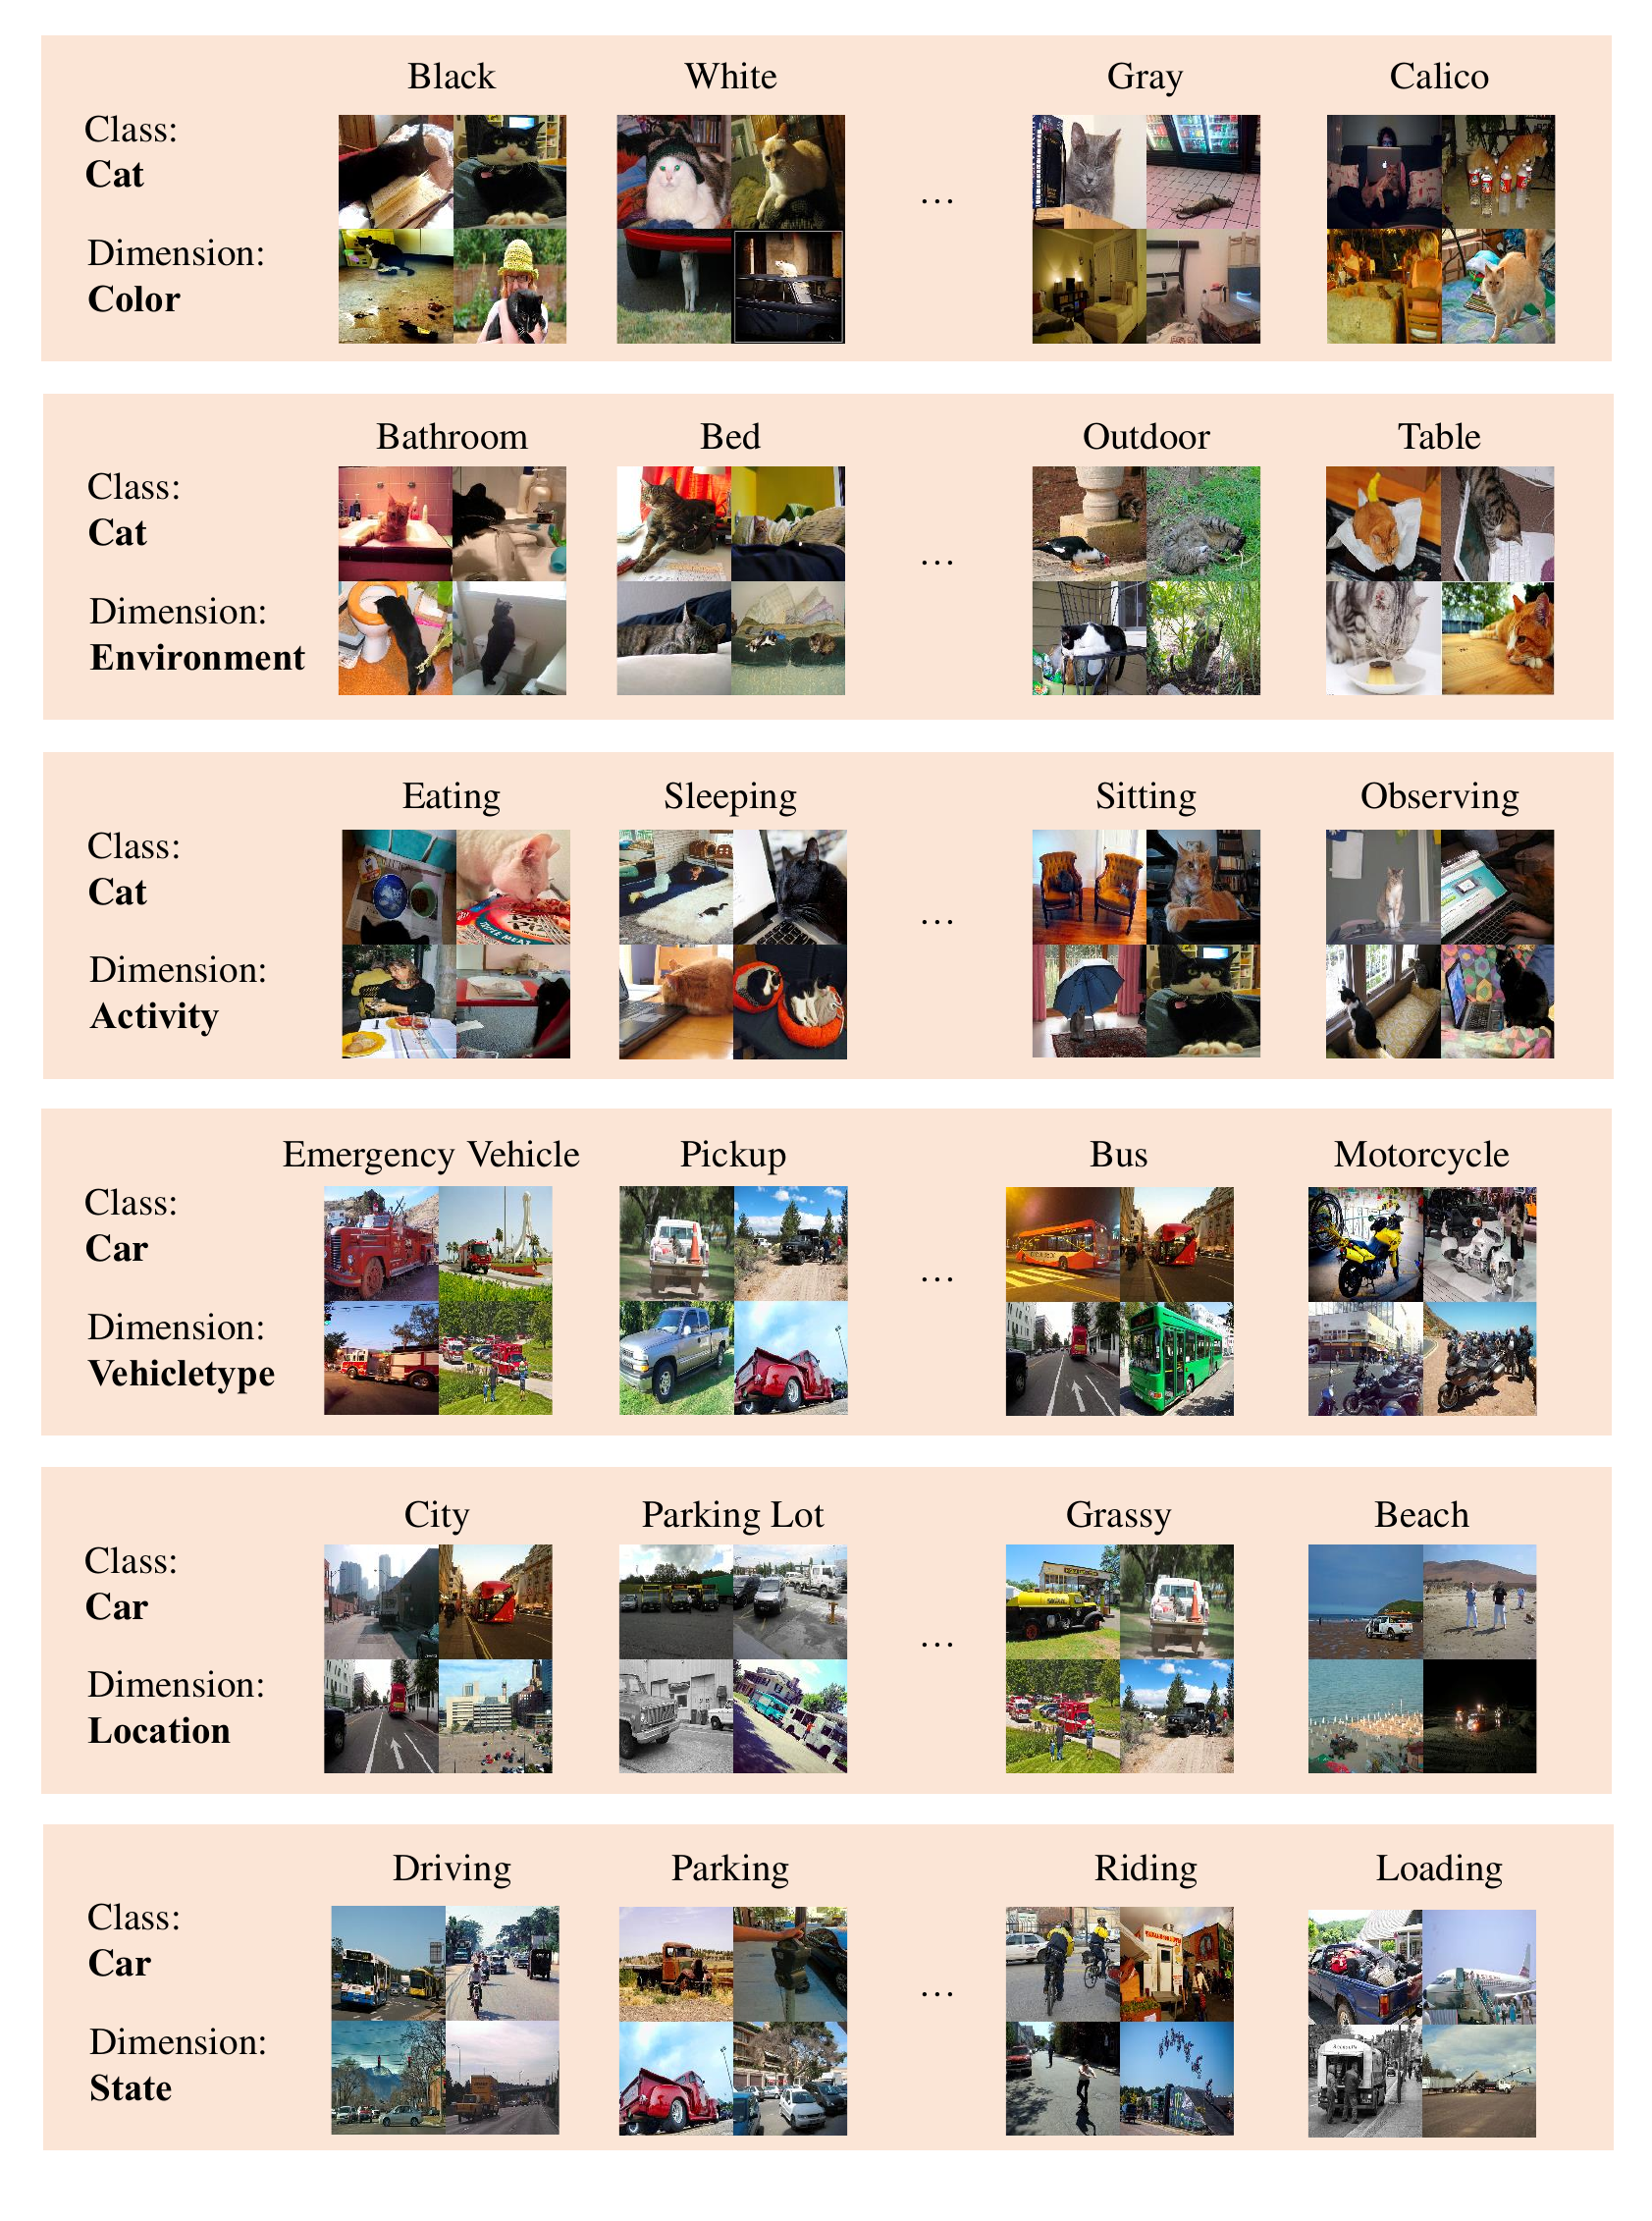}
    \caption{Visualizations of the discovered subpopulations with SSD-LLM.}
    \label{fig:appendix1}
    % \vspace{-0.4cm}
\end{figure}

\begin{figure}[H]
    \centering
    \includegraphics[width=1\linewidth]{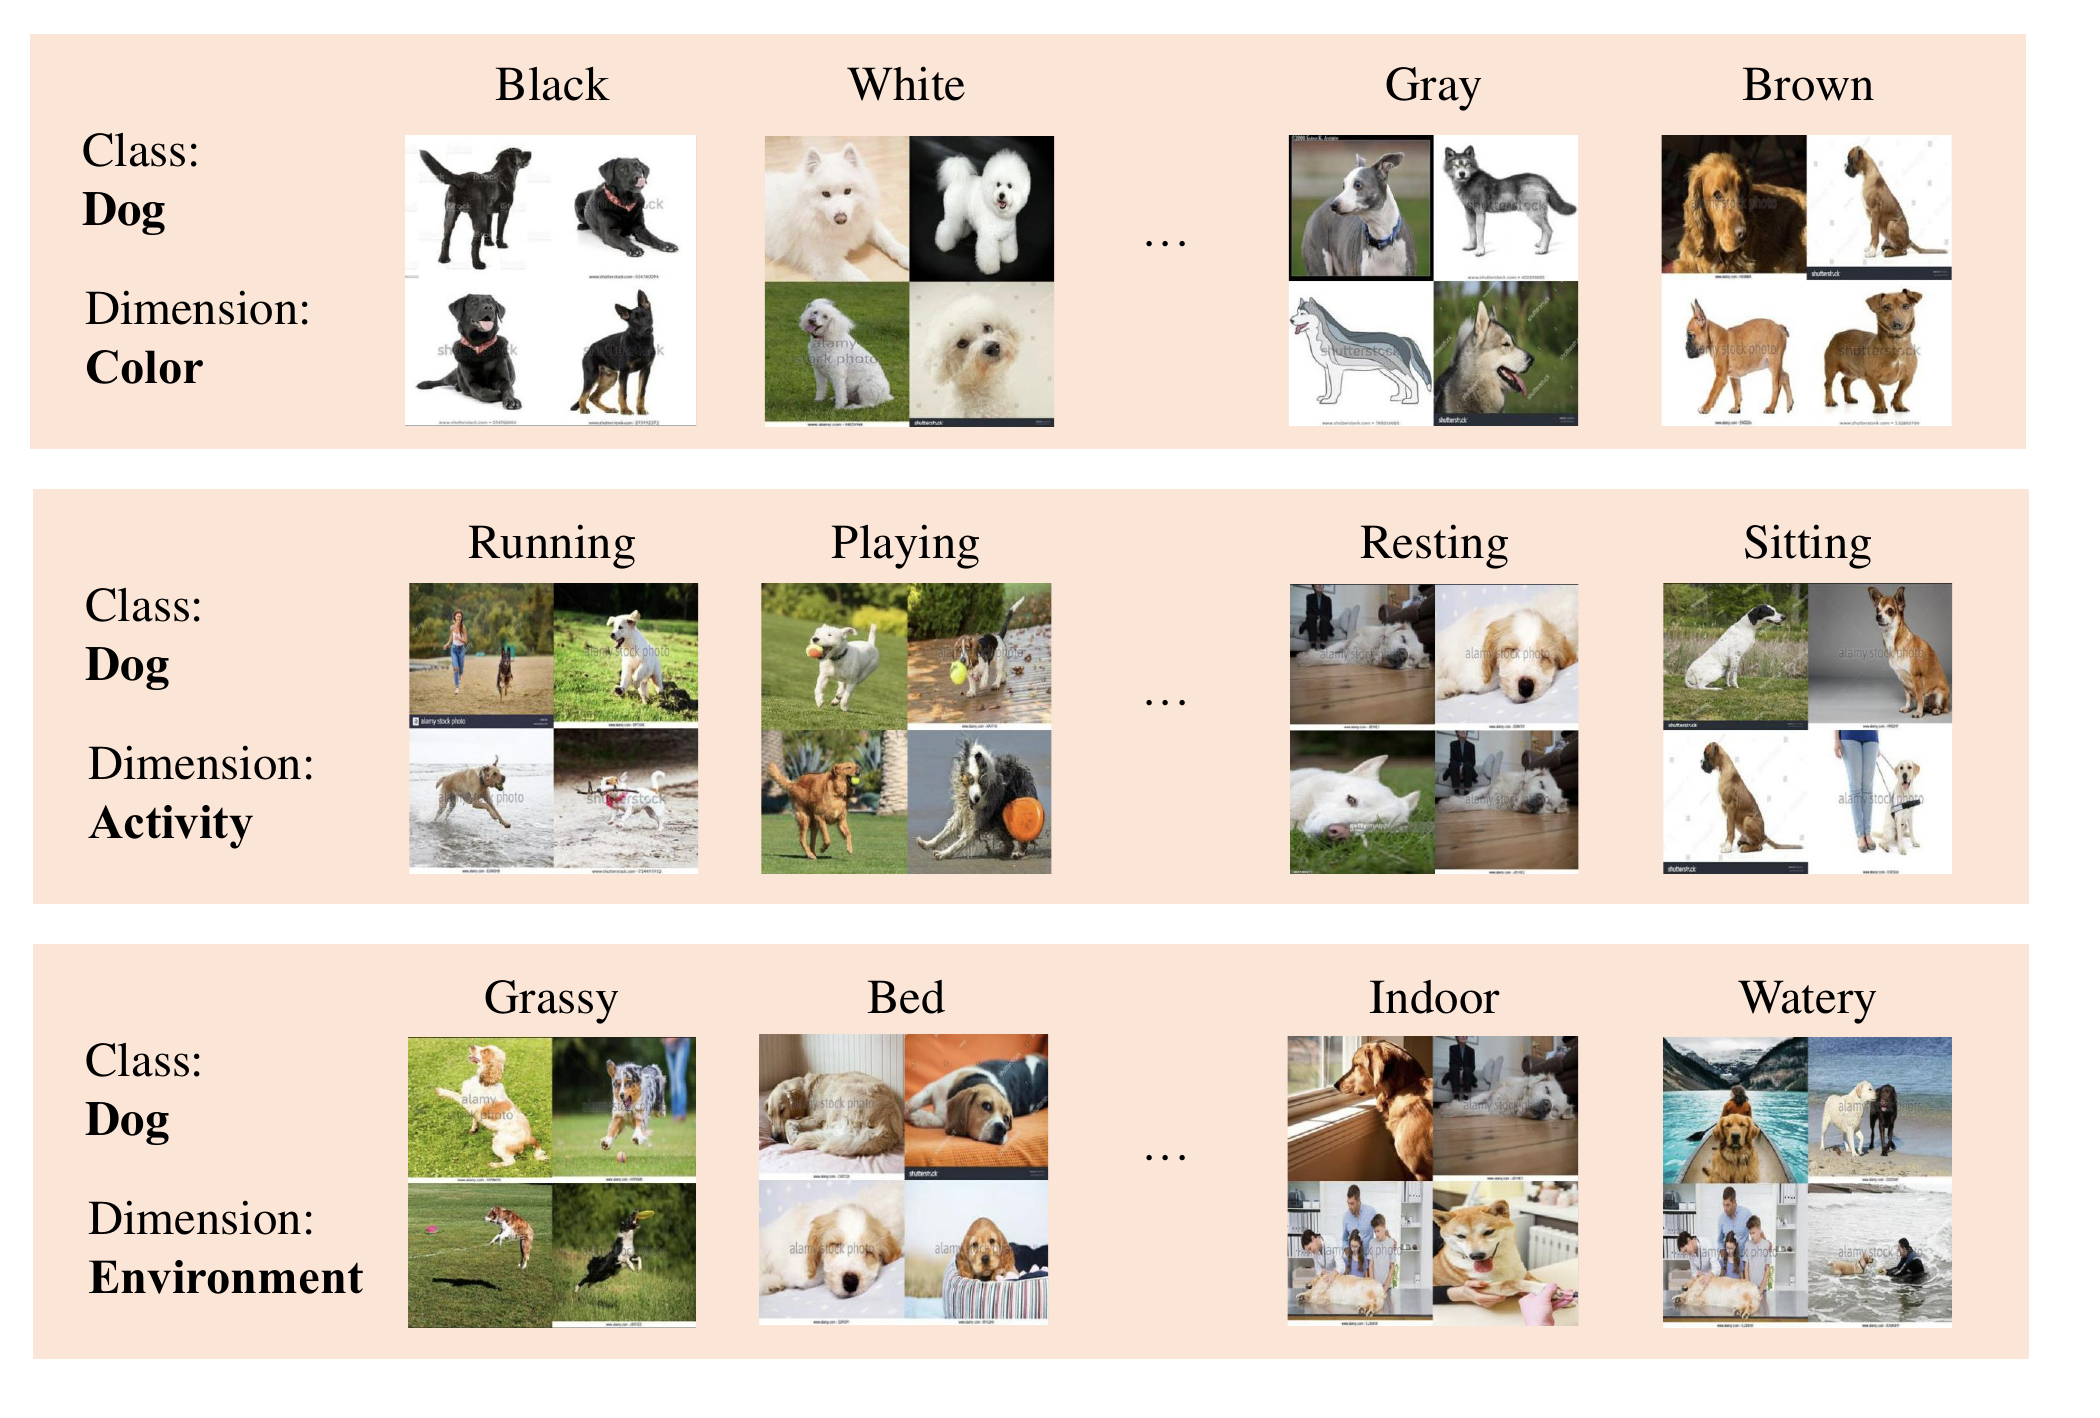}
    \caption{Visualizations of the discovered subpopulations with SSD-LLM.}
    \label{fig:appendix2}
    % \vspace{-0.6cm}
\end{figure}

\begin{figure}[H]
    \centering
    \includegraphics[width=1\linewidth]{fig/supp/crop_supp_dataset_organization(1).pdf}
    % \vspace{-0.6cm}
    \caption{Visualizations of the discovered slices with SSD-LLM.}
    \label{fig:appendix3}
    % \vspace{-0.6cm}
\end{figure}

\section{Pseudocode for Criteria Refinement}

% \vspace{-6mm}
\begin{algorithm}[H]
\caption*{\textbf{Step 3} Criteria Refinement}
\begin{algorithmic}[1]
\REQUIRE criteria: $Criteria$, Captions: $C$, Large language model: LLM
\ENSURE  Refined criteria: $Criteria$
\STATE \textbf{for} [$dim$, $Attributes$] \textbf{in} Criteria \textbf{do}
\STATE \quad\textbf{for} i \textbf{in range}(NumOfTests) \textbf{do}
\STATE \quad\quad\indent $c$ = $C$.sample()
\STATE \quad\quad\indent $Results$.append(LLM([$P_3^1$, $c$ $dim$, $attribute$]))
\STATE \quad\textbf{end for}
\STATE \quad\textbf{if} not Consistent($Results$)
\STATE \quad\quad\textbf{for} i \textbf{in range}(NumOfSuggests) \textbf{do}
\STATE \quad\quad\quad\indent $S$.append(LLM([$P_3^2$, $c$, $dim$, $attribute$]))
\STATE \quad\quad\textbf{end for}
\STATE \quad\quad $n$=LLMSummary($S$)
\STATE \quad\quad $Criteria[dim].append(n)$
\STATE \quad\quad $S$.reset()
\STATE \quad\textbf{end if}
\STATE \quad$Results$.reset()
\STATE \textbf{end for}
\end{algorithmic}
\end{algorithm}
% \subsubsection{Slice Discovery}
